# Supplementary material for: Multi-Player Bandits: A Trekking Approach
Source: arXiv:1809.06040 source file (2018-09-17)
Supplement: Supplementary file 1 [file Supplementary.tex]

%%%%%%%% ICML 2018 EXAMPLE LATEX SUBMISSION FILE %%%%%%%%%%%%%%%%%

\documentclass{article}


% Recommended, but optional, packages for figures and better typesetting:
\usepackage{microtype}
\usepackage{graphicx}
\usepackage{subfigure}
\usepackage{booktabs} % for professional tables
\usepackage{amsmath}
\usepackage{caption}
%\usepackage{subcaption}


%\usepackage[caption=false,font=footnotesize,labelfont=sf,textfont=sf]{subfig}
%\usepackage{algorithm}
%\usepackage{algorithmic}
%\usepackage{algpseudocode}
\usepackage{dblfloatfix}
%\usepackage[]{graphicx}
%\usepackage{cite}
%\usepackage{verbatim}
%\usepackage{url}
%\usepackage{amsmath}
%\usepackage{breqn}
%\usepackage{amsthm}
%\usepackage{multirow}
%%\usepackage{caption}
%\usepackage{lipsum}
%\usepackage{bbm}
%\usepackage{algorithm}
%\usepackage{algpseudocode}
%\usepackage[caption=false,font=footnotesize]{subfig}
%\usepackage{mathtools}
%\usepackage{amsmath,amsthm}
%\usepackage{amssymb,amsbsy,epsfig,float}
%\usepackage{graphicx,wrapfig,lipsum}

% hyperref makes hyperlinks in the resulting PDF.
% If your build breaks (sometimes temporarily if a hyperlink spans a page)
% please comment out the following usepackage line and replace
% \usepackage{icml2018} with \usepackage[nohyperref]{icml2018} above.
\usepackage{hyperref}

% Attempt to make hyperref and algorithmic work together better:
\newcommand{\theHalgorithm}{\arabic{algorithm}}
\newtheorem{defn}{Definition}
\newtheorem{thm}{Theorem}
\newtheorem{lemma}{Lemma}
\newtheorem{remark}{Remark]}

% Use the following line for the initial blind version submitted for review:
\usepackage{icml2018}

% If accepted, instead use the following line for the camera-ready submission:
%\usepackage[accepted]{icml2018}

% The \icmltitle you define below is probably too long as a header.
% Therefore, a short form for the running title is supplied here:
%\icmltitlerunning{Submission and Formatting Instructions for ICML 2018}

\begin{document}

\twocolumn[
\icmltitle{Supplementary for Multi-Player Bandits: A Trekking Approach}

% It is OKAY to include author information, even for blind
% submissions: the style file will automatically remove it for you
% unless you've provided the [accepted] option to the icml2018
% package.

% List of affiliations: The first argument should be a (short)
% identifier you will use later to specify author affiliations
% Academic affiliations should list Department, University, City, Region, Country
% Industry affiliations should list Company, City, Region, Country

% You can specify symbols, otherwise they are numbered in order.
% Ideally, you should not use this facility. Affiliations will be numbered
% in order of appearance and this is the preferred way.
%\icmlsetsymbol{equal}{*}
%
%\begin{icmlauthorlist}
%\icmlauthor{Aeiau Zzzz}{equal,to}
%\icmlauthor{Bauiu C.~Yyyy}{equal,to,goo}
%\icmlauthor{Cieua Vvvvv}{goo}
%\icmlauthor{Iaesut Saoeu}{ed}
%\icmlauthor{Fiuea Rrrr}{to}
%\icmlauthor{Tateu H.~Yasehe}{ed,to,goo}
%\icmlauthor{Aaoeu Iasoh}{goo}
%\icmlauthor{Buiui Eueu}{ed}
%\icmlauthor{Aeuia Zzzz}{ed}
%\icmlauthor{Bieea C.~Yyyy}{to,goo}
%\icmlauthor{Teoau Xxxx}{ed}
%\icmlauthor{Eee Pppp}{ed}
%\end{icmlauthorlist}
%
%\icmlaffiliation{to}{Department of Computation, University of Torontoland, Torontoland, Canada}
%\icmlaffiliation{goo}{Googol ShallowMind, New London, Michigan, USA}
%\icmlaffiliation{ed}{School of Computation, University of Edenborrow, Edenborrow, United Kingdom}
%
%\icmlcorrespondingauthor{Cieua Vvvvv}{c.vvvvv@googol.com}
%\icmlcorrespondingauthor{Eee Pppp}{ep@eden.co.uk}

% You may provide any keywords that you
% find helpful for describing your paper; these are used to populate
% the "keywords" metadata in the PDF but will not be shown in the document
\icmlkeywords{Multi-Player Bandits, Static and Dynamic set of Players}

\vskip 0.3in
]

% this must go after the closing bracket ] following \twocolumn[ ...

% This command actually creates the footnote in the first column
% listing the affiliations and the copyright notice.
% The command takes one argument, which is text to display at the start of the footnote.
% The \icmlEqualContribution command is standard text for equal contribution.
% Remove it (just {}) if you do not need this facility.

%\printAffiliationsAndNotice{}  % leave blank if no need to mention equal contribution
%\printAffiliationsAndNotice{\icmlEqualContribution} % otherwise use the standard text.

%\begin{abstract}
%We study stochastic multi-armed bandits with many players. The players do not know the number of players, cannot communicate with each other and if multiple players select a common arm they collide and none of them receive reward. We consider static scenario, where the number of players remains fixed, and the dynamic scenario, where the players enter and leave at any time. For both the scenarios we provide high probability algorithms based on a novel `trekking approach' that guarantees constant and sub-linear regret for the static and dynamic setting, respectively. The trekking approach eliminates the need to estimate number of players resulting in significant reduction in the number of collisions and improved regret performance compared to the state-of-the-art. We also develop an any-time algorithm that attains constant regret with high probability provided each player can 'sense' if another player has selected the same arm he wants to play. We validate our theoretical guarantees using simulation based and real test-bed based experiments.
%
%
% 
%\end{abstract}
%
%\section{Introduction}
%\label{submission}
%\input{Intro}
%
%\section{ Problem Setup}
%\label{setup}
%\input{Setup}
%
%\section{Algorithms and Analysis}
%\label{algorithms}
%\input{Algorithms}
%\section{Simulation Results}
%\label{SR}
%\input{simulation_results}
%\section{Appendix B: Simulation Results}
%\label{SR_extra}
%\input{simulation_results_ap}

%\label{Appendix}
\input{Appendix}



\section{Appendix B: Simulation Results}
\label{SR_extra}
\input{simulation_results_ap}

%\section{Format of the Paper}
%
%All submissions must follow the specified format.
%
%\subsection{Length and Dimensions}
%
%Papers must not exceed eight (8) pages, including all figures, tables,
%and appendices, but excluding references and acknowledgements. When references and acknowledgements are included,
%the paper must not exceed ten (10) pages.
%Acknowledgements should be limited to grants and people who contributed to the paper.
%Any submission that exceeds
%this page limit, or that diverges significantly from the specified format,
%will be rejected without review.
%
%The text of the paper should be formatted in two columns, with an
%overall width of 6.75~inches, height of 9.0~inches, and 0.25~inches
%between the columns. The left margin should be 0.75~inches and the top
%margin 1.0~inch (2.54~cm). The right and bottom margins will depend on
%whether you print on US letter or A4 paper, but all final versions
%must be produced for US letter size.
%
%The paper body should be set in 10~point type with a vertical spacing
%of 11~points. Please use Times typeface throughout the text.
%
%\subsection{Title}
%
%The paper title should be set in 14~point bold type and centered
%between two horizontal rules that are 1~point thick, with 1.0~inch
%between the top rule and the top edge of the page. Capitalize the
%first letter of content words and put the rest of the title in lower
%case.
%
%\subsection{Author Information for Submission}
%\label{author info}
%
%ICML uses double-blind review, so author information must not appear. If
%you are using \LaTeX\/ and the \texttt{icml2018.sty} file, use
%\verb+\icmlauthor{...}+ to specify authors and \verb+\icmlaffiliation{...}+ to specify affiliations. (Read the TeX code used to produce this document for an example usage.) The author information
%will not be printed unless \texttt{accepted} is passed as an argument to the
%style file.
%Submissions that include the author information will not
%be reviewed.
%
%\subsubsection{Self-Citations}
%
%If you are citing published papers for which you are an author, refer
%to yourself in the third person. In particular, do not use phrases
%that reveal your identity (e.g., ``in previous work \cite{langley00}, we
%have shown \ldots'').
%
%Do not anonymize citations in the reference section. The only exception are manuscripts that are
%not yet published (e.g., under submission). If you choose to refer to
%such unpublished manuscripts \cite{anonymous}, anonymized copies have
%to be submitted
%as Supplementary Material via CMT\@. However, keep in mind that an ICML
%paper should be self contained and should contain sufficient detail
%for the reviewers to evaluate the work. In particular, reviewers are
%not required to look at the Supplementary Material when writing their
%review.
%
%\subsubsection{Camera-Ready Author Information}
%\label{final author}
%
%If a paper is accepted, a final camera-ready copy must be prepared.
%%
%For camera-ready papers, author information should start 0.3~inches below the
%bottom rule surrounding the title. The authors' names should appear in 10~point
%bold type, in a row, separated by white space, and centered. Author names should
%not be broken across lines. Unbolded superscripted numbers, starting 1, should
%be used to refer to affiliations.
%
%Affiliations should be numbered in the order of appearance. A single footnote
%block of text should be used to list all the affiliations. (Academic
%affiliations should list Department, University, City, State/Region, Country.
%Similarly for industrial affiliations.)
%
%Each distinct affiliations should be listed once. If an author has multiple
%affiliations, multiple superscripts should be placed after the name, separated
%by thin spaces. If the authors would like to highlight equal contribution by
%multiple first authors, those authors should have an asterisk placed after their
%name in superscript, and the term ``\textsuperscript{*}Equal contribution"
%should be placed in the footnote block ahead of the list of affiliations. A
%list of corresponding authors and their emails (in the format Full Name
%\textless{}email@domain.com\textgreater{}) can follow the list of affiliations.
%Ideally only one or two names should be listed.
%
%A sample file with author names is included in the ICML2018 style file
%package. Turn on the \texttt{[accepted]} option to the stylefile to
%see the names rendered. All of the guidelines above are implemented
%by the \LaTeX\ style file.
%
%\subsection{Abstract}
%
%The paper abstract should begin in the left column, 0.4~inches below the final
%address. The heading `Abstract' should be centered, bold, and in 11~point type.
%The abstract body should use 10~point type, with a vertical spacing of
%11~points, and should be indented 0.25~inches more than normal on left-hand and
%right-hand margins. Insert 0.4~inches of blank space after the body. Keep your
%abstract brief and self-contained, limiting it to one paragraph and roughly 4--6
%sentences. Gross violations will require correction at the camera-ready phase.
%
%\subsection{Partitioning the Text}
%
%You should organize your paper into sections and paragraphs to help
%readers place a structure on the material and understand its
%contributions.
%
%\subsubsection{Sections and Subsections}
%
%Section headings should be numbered, flush left, and set in 11~pt bold
%type with the content words capitalized. Leave 0.25~inches of space
%before the heading and 0.15~inches after the heading.
%
%Similarly, subsection headings should be numbered, flush left, and set
%in 10~pt bold type with the content words capitalized. Leave
%0.2~inches of space before the heading and 0.13~inches afterward.
%
%Finally, subsubsection headings should be numbered, flush left, and
%set in 10~pt small caps with the content words capitalized. Leave
%0.18~inches of space before the heading and 0.1~inches after the
%heading.
%
%Please use no more than three levels of headings.
%
%\subsubsection{Paragraphs and Footnotes}
%
%Within each section or subsection, you should further partition the
%paper into paragraphs. Do not indent the first line of a given
%paragraph, but insert a blank line between succeeding ones.
%
%You can use footnotes\footnote{Footnotes
%should be complete sentences.} to provide readers with additional
%information about a topic without interrupting the flow of the paper.
%Indicate footnotes with a number in the text where the point is most
%relevant. Place the footnote in 9~point type at the bottom of the
%column in which it appears. Precede the first footnote in a column
%with a horizontal rule of 0.8~inches.\footnote{Multiple footnotes can
%appear in each column, in the same order as they appear in the text,
%but spread them across columns and pages if possible.}
%
%\begin{figure}[ht]
%\vskip 0.2in
%\begin{center}
%\centerline{\includegraphics[width=\columnwidth]{icml_numpapers}}
%\caption{Historical locations and number of accepted papers for International
%Machine Learning Conferences (ICML 1993 -- ICML 2008) and International
%Workshops on Machine Learning (ML 1988 -- ML 1992). At the time this figure was
%produced, the number of accepted papers for ICML 2008 was unknown and instead
%estimated.}
%\label{icml-historical}
%\end{center}
%\vskip -0.2in
%\end{figure}
%
%\subsection{Figures}
%
%You may want to include figures in the paper to illustrate
%your approach and results. Such artwork should be centered,
%legible, and separated from the text. Lines should be dark and at
%least 0.5~points thick for purposes of reproduction, and text should
%not appear on a gray background.
%
%Label all distinct components of each figure. If the figure takes the
%form of a graph, then give a name for each axis and include a legend
%that briefly describes each curve. Do not include a title inside the
%figure; instead, the caption should serve this function.
%
%Number figures sequentially, placing the figure number and caption
%\emph{after} the graphics, with at least 0.1~inches of space before
%the caption and 0.1~inches after it, as in
%Figure~\ref{icml-historical}. The figure caption should be set in
%9~point type and centered unless it runs two or more lines, in which
%case it should be flush left. You may float figures to the top or
%bottom of a column, and you may set wide figures across both columns
%(use the environment \texttt{figure*} in \LaTeX). Always place
%two-column figures at the top or bottom of the page.
%
%\subsection{Algorithms}
%
%If you are using \LaTeX, please use the ``algorithm'' and ``algorithmic''
%environments to format pseudocode. These require
%the corresponding stylefiles, algorithm.sty and
%algorithmic.sty, which are supplied with this package.
%Algorithm~\ref{alg:example} shows an example.
%
%\begin{algorithm}[tb]
%   \caption{Bubble Sort}
%   \label{alg:example}
%\begin{algorithmic}
%   \STATE {\bfseries Input:} data $x_i$, size $m$
%   \REPEAT
%   \STATE Initialize $noChange = true$.
%   \FOR{$i=1$ {\bfseries to} $m-1$}
%   \IF{$x_i > x_{i+1}$}
%   \STATE Swap $x_i$ and $x_{i+1}$
%   \STATE $noChange = false$
%   \ENDIF
%   \ENDFOR
%   \UNTIL{$noChange$ is $true$}
%\end{algorithmic}
%\end{algorithm}
%
%\subsection{Tables}
%
%You may also want to include tables that summarize material. Like
%figures, these should be centered, legible, and numbered consecutively.
%However, place the title \emph{above} the table with at least
%0.1~inches of space before the title and the same after it, as in
%Table~\ref{sample-table}. The table title should be set in 9~point
%type and centered unless it runs two or more lines, in which case it
%should be flush left.
%
%% Note use of \abovespace and \belowspace to get reasonable spacing
%% above and below tabular lines.
%
%\begin{table}[t]
%\caption{Classification accuracies for naive Bayes and flexible
%Bayes on various data sets.}
%\label{sample-table}
%\vskip 0.15in
%\begin{center}
%\begin{small}
%\begin{sc}
%\begin{tabular}{lcccr}
%\toprule
%Data set & Naive & Flexible & Better? \\
%\midrule
%Breast    & 95.9$\pm$ 0.2& 96.7$\pm$ 0.2& $\surd$ \\
%Cleveland & 83.3$\pm$ 0.6& 80.0$\pm$ 0.6& $\times$\\
%Glass2    & 61.9$\pm$ 1.4& 83.8$\pm$ 0.7& $\surd$ \\
%Credit    & 74.8$\pm$ 0.5& 78.3$\pm$ 0.6&         \\
%Horse     & 73.3$\pm$ 0.9& 69.7$\pm$ 1.0& $\times$\\
%Meta      & 67.1$\pm$ 0.6& 76.5$\pm$ 0.5& $\surd$ \\
%Pima      & 75.1$\pm$ 0.6& 73.9$\pm$ 0.5&         \\
%Vehicle   & 44.9$\pm$ 0.6& 61.5$\pm$ 0.4& $\surd$ \\
%\bottomrule
%\end{tabular}
%\end{sc}
%\end{small}
%\end{center}
%\vskip -0.1in
%\end{table}
%
%Tables contain textual material, whereas figures contain graphical material.
%Specify the contents of each row and column in the table's topmost
%row. Again, you may float tables to a column's top or bottom, and set
%wide tables across both columns. Place two-column tables at the
%top or bottom of the page.
%
%\subsection{Citations and References}
%
%Please use APA reference format regardless of your formatter
%or word processor. If you rely on the \LaTeX\/ bibliographic
%facility, use \texttt{natbib.sty} and \texttt{icml2018.bst}
%included in the style-file package to obtain this format.
%
%Citations within the text should include the authors' last names and
%year. If the authors' names are included in the sentence, place only
%the year in parentheses, for example when referencing Arthur Samuel's
%pioneering work \yrcite{Samuel59}. Otherwise place the entire
%reference in parentheses with the authors and year separated by a
%comma \cite{Samuel59}. List multiple references separated by
%semicolons \cite{kearns89,Samuel59,mitchell80}. Use the `et~al.'
%construct only for citations with three or more authors or after
%listing all authors to a publication in an earlier reference \cite{MachineLearningI}.
%
%Authors should cite their own work in the third person
%in the initial version of their paper submitted for blind review.
%Please refer to Section~\ref{author info} for detailed instructions on how to
%cite your own papers.
%
%Use an unnumbered first-level section heading for the references, and use a
%hanging indent style, with the first line of the reference flush against the
%left margin and subsequent lines indented by 10 points. The references at the
%end of this document give examples for journal articles \cite{Samuel59},
%conference publications \cite{langley00}, book chapters \cite{Newell81}, books
%\cite{DudaHart2nd}, edited volumes \cite{MachineLearningI}, technical reports
%\cite{mitchell80}, and dissertations \cite{kearns89}.
%
%Alphabetize references by the surnames of the first authors, with
%single author entries preceding multiple author entries. Order
%references for the same authors by year of publication, with the
%earliest first. Make sure that each reference includes all relevant
%information (e.g., page numbers).
%
%Please put some effort into making references complete, presentable, and
%consistent. If using bibtex, please protect capital letters of names and
%abbreviations in titles, for example, use \{B\}ayesian or \{L\}ipschitz
%in your .bib file.
%
%\subsection{Software and Data}
%
%We strongly encourage the publication of software and data with the
%camera-ready version of the paper whenever appropriate. This can be
%done by including a URL in the camera-ready copy. However, do not
%include URLs that reveal your institution or identity in your
%submission for review. Instead, provide an anonymous URL or upload
%the material as ``Supplementary Material'' into the CMT reviewing
%system. Note that reviewers are not required to look a this material
%when writing their review.
%
%% Acknowledgements should only appear in the accepted version.
%\section*{Acknowledgements}
%
%\textbf{Do not} include acknowledgements in the initial version of
%the paper submitted for blind review.
%
%If a paper is accepted, the final camera-ready version can (and
%probably should) include acknowledgements. In this case, please
%place such acknowledgements in an unnumbered section at the
%end of the paper. Typically, this will include thanks to reviewers
%who gave useful comments, to colleagues who contributed to the ideas,
%and to funding agencies and corporate sponsors that provided financial
%support.
%
%
%% In the unusual situation where you want a paper to appear in the
%% references without citing it in the main text, use \nocite
%\nocite{langley00}
%
\bibliography{biblio}
\bibliographystyle{icml2018}
%
%
%%%%%%%%%%%%%%%%%%%%%%%%%%%%%%%%%%%%%%%%%%%%%%%%%%%%%%%%%%%%%%%%%%%%%%%%%%%%%%%%
%%%%%%%%%%%%%%%%%%%%%%%%%%%%%%%%%%%%%%%%%%%%%%%%%%%%%%%%%%%%%%%%%%%%%%%%%%%%%%%%
%% DELETE THIS PART. DO NOT PLACE CONTENT AFTER THE REFERENCES!
%%%%%%%%%%%%%%%%%%%%%%%%%%%%%%%%%%%%%%%%%%%%%%%%%%%%%%%%%%%%%%%%%%%%%%%%%%%%%%%%
%%%%%%%%%%%%%%%%%%%%%%%%%%%%%%%%%%%%%%%%%%%%%%%%%%%%%%%%%%%%%%%%%%%%%%%%%%%%%%%%
%\appendix
%\section{Do \emph{not} have an appendix here}
%
%\textbf{\emph{Do not put content after the references.}}
%%
%Put anything that you might normally include after the references in a separate
%supplementary file.
%
%We recommend that you build supplementary material in a separate document.
%If you must create one PDF and cut it up, please be careful to use a tool that
%doesn't alter the margins, and that doesn't aggressively rewrite the PDF file.
%pdftk usually works fine. 
%
%\textbf{Please do not use Apple's preview to cut off supplementary material.} In
%previous years it has altered margins, and created headaches at the camera-ready
%stage. 
%%%%%%%%%%%%%%%%%%%%%%%%%%%%%%%%%%%%%%%%%%%%%%%%%%%%%%%%%%%%%%%%%%%%%%%%%%%%%%%%
%%%%%%%%%%%%%%%%%%%%%%%%%%%%%%%%%%%%%%%%%%%%%%%%%%%%%%%%%%%%%%%%%%%%%%%%%%%%%%%%
%

\end{document}


% This document was modified from the file originally made available by
% Pat Langley and Andrea Danyluk for ICML-2K. This version was created
% by Iain Murray in 2018. It was modified from a version from Dan Roy in
% 2017, which was based on a version from Lise Getoor and Tobias
% Scheffer, which was slightly modified from the 2010 version by
% Thorsten Joachims & Johannes Fuernkranz, slightly modified from the
% 2009 version by Kiri Wagstaff and Sam Roweis's 2008 version, which is
% slightly modified from Prasad Tadepalli's 2007 version which is a
% lightly changed version of the previous year's version by Andrew
% Moore, which was in turn edited from those of Kristian Kersting and
% Codrina Lauth. Alex Smola contributed to the algorithmic style files.
